# Supplementary material for: Repulsion, Chaos and Equilibrium in Mixture Models
Source: arXiv:2306.10669 source file (2023-06-19)
Supplement: Supplementary file 1 [file RepMix_SM.pdf]

# Repulsion, Chaos and Equilibrium in Mixture Models
# Supplementary Material

Andrea Cremaschi[1,2], Timothy M. Wertz[3], and Maria De Iorio[1,2,4]

[1]Singapore Institute for Clinical Sciences (SICS), Agency for Science, Technology and Research (A*STAR), Singapore, Republic of Singapore
[2]Department of Paediatrics, Yong Loo Lin School of Medicine, National University of Singapore (NUS), Singapore, Republic of Singapore
[3]Department of Mathematics, National University of Singapore (NUS), Singapore, Republic of Singapore
[4]Department of Statistical Science, University College London (UCL), London, UK

## Abstract

This document contains the Supplementary Material information for the manuscript *Repulsion, Chaos and Equilibrium in Mixture Models.* We present in Section 1 the steps of the Gibbs sampling algorithm used to perform posterior inference under the proposed model.

## 1 MCMC algorithm

We present in this section the MCMC algorithm used to perform posterior inference with the proposed model. The algorithm follows the scheme of Beraha et al. [2022], where a birth and death Metropolis-within-Gibbs step is used to update the components in the model not associated with any observations (i.e., empty).

For clarity of exposition, we report here the full model specification:

$$
\begin{aligned}
&\boldsymbol{y}_i \mid z_i, \boldsymbol{\theta}, M \sim f(\boldsymbol{y}_i \mid \boldsymbol{\theta}_{z_i}) \quad i = 1, \ldots, N \\
&\boldsymbol{\theta}_1, \ldots, \boldsymbol{\theta}_M \mid M \sim P_0(\boldsymbol{\theta}) \\
&\mathbb{P}(z_i = h \mid \boldsymbol{S}, M) \propto S_h \quad h = 1, \ldots, M \\
&S_1, \ldots, S_M \mid M \overset{\text{iid}}{\sim} \text{Gamma}(\gamma_S, 1) \\
&M \sim \text{Poi}_1(\Lambda)
\end{aligned} \tag{1}
$$

where Gamma$(a, b)$ represents the Gamma distribution with mean $a/b$ and variance $a/b^2$, while $\text{Poi}_1(\Lambda)$ is the Poisson distribution shifted by one unit, i.e. the random variable $M - 1$ is Poisson with mean $\Lambda$.

Let $M^{(a)}, M^{(na)}$ be the sets of components associated and not associated with observations, respectively. We indicate with $K_N = |M^{(a)}|$ the number of clusters, to which correspond the cluster sizes $n_1, \ldots, n_{K_N}$. Similarly, we split the vector of location parameters into $\boldsymbol{\theta} = \left(\boldsymbol{\theta}^{(a)}, \boldsymbol{\theta}^{(na)}\right)$. Following Argiento and De Iorio [2022], given the location parameters $\boldsymbol{\theta}$ and an auxiliary variable $u$, we can write the joint law of the normalised finite point process as follows:

$$
\begin{aligned}
&\mathcal{L}(P \mid u, \boldsymbol{\theta}) \propto \mathcal{L}(P, u \mid \boldsymbol{\theta}) \propto \\
&\left(\prod_{m \in M^{(a)}} S_m^{n_m} \delta_{\boldsymbol{\theta}^\star}(\boldsymbol{\theta}^\star_m)\right) \left(M^{(na)} + K_N\right)! p(M^{(na)} + K_N) \left(\prod_{m=1}^{M} e^{-u S_m} \text{gamma}(S_m \mid \gamma_S, 1)\right) P_0(\boldsymbol{\theta}) = \\
&\left(\prod_{m \in M^{(a)}} S_m^{n_m} \delta_{\boldsymbol{\theta}^\star}(\boldsymbol{\theta}^\star_m) e^{-u S_m} \text{gamma}(S_m \mid \gamma_S, 1) P_0(\boldsymbol{\theta}^{(a)})\right) \qquad (2) \\
&\left(M^{(na)} + K_N\right)! p(M^{(na)} + K_N) \left(\prod_{m \in M^{(na)}} e^{-u S_m} \text{gamma}(S_m \mid \gamma_S, 1) P_0(\boldsymbol{\theta}^{(na)} \mid \boldsymbol{\theta}^{(a)})\right) = \\
&\mathcal{L}(P^{(na)} \mid u, \boldsymbol{\theta}^{(na)}, \boldsymbol{\theta}^{(a)}) \mathcal{L}(P^{(a)} \mid u, \boldsymbol{\theta}^{(a)})
\end{aligned}
$$

showing that the finite point process can still be factorised, a key point in the development of the algorithm in Argiento and De Iorio [2022], although here it is done in a conditional way. This implies that the algorithm part where the empty components are updated needs to be performed conditionally on the non-empty ones.

We provide now the steps of the algorithm:

- Update the allocation parameters $\boldsymbol{z} = (z_1, \ldots, z_N)$. For each $i = 1, \ldots, N$, sample:

$$
p\left(z_i = h \mid \boldsymbol{S}, M, \boldsymbol{y}_i\right) \propto S_h f\left(\boldsymbol{y}_i \mid \boldsymbol{\theta}^\star_h\right), \quad h = 1, \ldots, M
$$

- Update the unnormalised weights from:

$$
\begin{aligned}
S_m \mid M, \boldsymbol{z}, \gamma_S, u &\sim \text{Gamma}(\gamma_S, n_m), && m = 1, \ldots, K_N \\
S_m \mid M, \boldsymbol{z}, \gamma_S, u &\sim \text{Gamma}(\gamma_S, 1), && m = K_N + 1, \ldots, M
\end{aligned}
$$

- Update the auxiliary variable $u \sim \text{Gamma}\left(\sum_{m=1}^{M} S_m, N\right)$

- Update the location parameters $\boldsymbol{\theta}^{(a)}$ from the following full-conditional:

$$
p\left(\boldsymbol{\theta}_j^{(a)} \mid \boldsymbol{y}, \boldsymbol{z}\right) \propto \left(\prod_{i \in C_j} f\left(\boldsymbol{y}_i \mid \boldsymbol{\theta}_j\right)\right) P_0\left(\boldsymbol{\theta}^{(a)}, \boldsymbol{\theta}^{(na)}\right)
$$

  This update can be performed via a Metropolis-Hastings step.

- Update jointly the location parameters $\boldsymbol{\theta}^{(na)}$ and the number of empty components $M^{(na)}$ from the following full-conditional (from Eq. (2)):

$$
p\left(\boldsymbol{\theta}_j^{(na)}, M^{(na)} \mid \boldsymbol{\theta}^{(a)}, u\right) \propto \tag{3}
$$
$$
\left(\prod_{m \in M^{(na)}} e^{-uS_m} \text{Gamma}\left(S_m \mid \gamma_S, 1\right)\right) P_0\left(\boldsymbol{\theta}^{(a)}, \boldsymbol{\theta}^{(na)}\right) p\left(M^{(na)} + K_N\right)
$$

  By marginalising the unnormalised weights, and exploiting the Laplace transform $\Psi(u) = \int_0^{+\infty} e^{-uS_m} \text{Gamma}(S_m \mid \gamma_S, 1) dS_m = (u+1)^{-1}$, we have:

$$
\begin{aligned}
&p\left(\boldsymbol{\theta}_j^{(na)}, M^{(na)} \mid \boldsymbol{\theta}^{(a)}, u\right) \propto \\
&\Psi(u)^{M^{(na)}} P_0\left(\boldsymbol{\theta}^{(a)}, \boldsymbol{\theta}^{(na)}\right) p\left(M^{(na)} + K_N\right)
\end{aligned} \tag{4}
$$

  The latter marginalisation is very important as it allows to get rid of the additional terms relative to the unnormalised weights, improving computations.

  To sample from this full-conditional, we need to perform a trans-dimensional move, since at each iteration the number of non-allocated components is allowed to change. Following Beraha et al. [2022], we use birth-and-death Metropolis-Hastings step, where at each proposal only one component of the mixture is changed (added or removed). Let $p_b$ and $p_d$, with $p_b + p_d = 1$, be the probability of performing a birth or a death move, respectively. These values are fixed beforehand, unless $M^{(na)} = 0$ in the current move, and then $p_b = 1$ and $p_d = 0$. When a birth move is selected, a new value for the location of a new empty component is proposed. When a death move is selected, one of the existing empty components chosen uniformly at random is deleted from the mixture.

- Birth move: propose a new value for $\boldsymbol{\theta}_{M+1} \sim q\left(\boldsymbol{\theta} \mid \boldsymbol{\theta}_{1:M}\right)$ and accept the resulting configuration with probability:

$$\min\left\{1, \frac{P_0(\boldsymbol{\theta}_{1:M+1})}{P_0(\boldsymbol{\theta}_{1:M})} \frac{\Psi(u)^{M^{(na)}+1}}{\Psi(u)^{M^{(na)}}} \frac{p_d \frac{1}{M^{(na)}+1}}{p_b q\left(\boldsymbol{\theta}_{M+1} \mid \boldsymbol{\theta}_{1:M}\right)} \frac{p(M+1)}{p(M)}\right\}$$

where the term $\frac{1}{(M^{(na)}+1)}$ comes from the reverse death move, in which we select one of the empty components uniformly at random to be deleted.

- Death move: select one of the empty components uniformly at random to be deleted and accept this configuration with probability:

$$\min\left\{1, \frac{P_0(\boldsymbol{\theta}_{1:M-1})}{P_0(\boldsymbol{\theta}_{1:M})} \frac{\Psi(u)^{M^{(na)}-1}}{\Psi(u)^{M^{(na)}}} \frac{p_b q\left(\boldsymbol{\theta}_M \mid \boldsymbol{\theta}_{1:M-1}\right)}{p_d \frac{1}{M^{(na)}}} \frac{p(M-1)}{p(M)}\right\}$$

In the proposed framework, the joint distribution for the location parameters $\boldsymbol{\theta}$ has a tractable form and allows for the evaluation of the above ratios. Furthermore, selecting an appropriate proposal distribution would lead to further cancellations in the acceptance probability ratios. For instance, a suitable choice would be to use the one-dimensional version of the proposed joint densities derived from those of the eigenvalues of the Gaussian, Wishart and Beta matrices, which are simply Normal, Gamma and Beta distributions, respectively.

- Update hyperparameters of the repulsive distribution. Let $Z_M(\alpha, \beta, \zeta)$ represent the normalising constant for the distributions under study. Since this value is known in closed form, we can perform a Metropolis-Hastings update targeting the following full-conditional:

$$p\left(\alpha \mid \boldsymbol{\theta}, M, \beta, \zeta\right) \propto P_0\left(\boldsymbol{\theta} \mid \alpha, \beta, \zeta\right) p\left(\alpha\right)$$

and similarly for $\beta$ and $\zeta$. Note that the expression of $Z_M\left(\alpha, \beta, \zeta\right)$ enters the definition of $P_0\left(\boldsymbol{\theta} \mid \alpha, \beta, \zeta\right)$ in the expression above. Note that we can also specify joint prior distributions for these parameters, as long as they satisfy the necessary constraint required to ensure that the joint eigenvalue distributions are well-defined.

# References

Raffaele Argiento and Maria De Iorio. Is infinity that far? a bayesian nonparametric perspective of finite mixture models. *The Annals of Statistics*, 50(5): 2641–2663, 2022.

Mario Beraha, Raffaele Argiento, Jesper Møller, and Alessandra Guglielmi. Mcmc computations for bayesian mixture models using repulsive point processes. *Journal of Computational and Graphical Statistics*, pages 1–14, 2022.
